# Supplementary material for: Time-Aware Tensor Decomposition for Missing Entry Prediction
Source: arXiv:2012.08855 source file (2020-12-16)
Supplement: Supplementary file 1 [file 070appendix1.tex]

\subsection{Extra experiment on datasets from data center} \label{subsec:datacenter}

\begin{table}
	\centering
	\vspace{5mm}
	\begin{threeparttable}
	\caption{
		\label{tab:datacenter_dataset}
		Summary of real-world tensors from data center. Bold text denotes time mode.
	}
	\begin{tabular}{ l c r r c}
		\toprule
		\textbf{Name} & \textbf{Dimensionality} & \textbf{Nonzero} &\textbf{Density}\\
		\midrule
	    server room \tnote{1} & 3 $\times$ 3 $\times$ 34 $\times$ \bf{4,157} & 1,009,426 & $7.935e-01$ \\ 	
%	   	Google cluster\tnote{2} & {\bf 76} $\times$ 176,580 $\times$ 9,218 & 3,535,029 & $2.857e-05$ \\ 	
	    \bottomrule
	\end{tabular}
	\scriptsize
	\begin{tablenotes}
	\item[1] {\url{https://zenodo.org/record/3610078#.XlNpAigzaM8}}
%	\item[2] {\url{https://github.com/google/cluster-data}}
\end{tablenotes}
\end{threeparttable}	
\end{table}

\begin{itemize}
	\item server room
	is a 4-mode tensor (cooling, power usage, location, second) containing temperature.
	\item Mode 1 : air conditioning temperature setups (24, 27 and 30 Celsius degrees)
	\item Mode 2 : power usage ($50\%, 75\%, 100\%$ scenario)
	\item Mode 3 : temperature probes
	\item Mode 4 : duration time (3000~4000s)
\end{itemize}
	
%\begin{itemize}
%	\item Google cluster
%	is a 3-mode tensor (seconds, job id, task id) containing memory consumed by a task during seven hours.
%	The data consists of a set of tasks, where each task runs on a single machine. 
%	Each task belongs to a single job; a job may have multiple tasks (e.g., mappers and reducers).
%	The data have been anonymized in several ways: 
%		there are no task or job names, just numeric identifiers; 
%		timestamps are relative to the start of data collection; 
%		the consumption of CPU and memory is obscured using a linear transformation. 
		
%\end{itemize}

\begin{table}
	\small
	\centering
	\caption{
	Performance of missing entry prediction by TATD and competitors on a data center dataset.
	The best is in bold, and the second-best method is underlined.
	}	
	\setlength{\tabcolsep}{12pt} 	
	\begin{tabular}{l | cc }
		\toprule
		Data &
		\multicolumn{2}{c}{\makecell{server room \\ (z-score normalization)}} \\
	    \midrule
		\diagbox[height=2em]{Method}{Metric}
		& RMSE & MAE
		\\ \midrule
		\cpals~\cite{harshman1970foundations}
		& 0.076 & 0.030  \\ [0.3em]
		CoSTCo~\cite{liu2019costco}
		& 0.675 & 0.387 \\ [0.3em]
		TRMF~\cite{yu2016temporal}
		& 1.083 & 0.8134 \\ [0.3em]
		NTF~\cite{wu2019neural}
		& 0.660 & 0.516 \\ [0.3em]
		\midrule
		\methodz
		& \underline{0.058} & \underline{0.039} \\ [0.3em]
		\bf{\method}
		&  \bf{0.054} & \bf{0.035}
		\\
	\bottomrule
	\end{tabular}
	\label{tab:appendix_exp}
\end{table}

%\begin{table}
%	\small
%	\centering
%	\caption{
%	Performance of missing entry prediction by TATD and competitors on a data center dataset.
%	The best is in bold, and the second-best method is underlined.
%	}	
%	\setlength{\tabcolsep}{12pt} 	
%	\begin{tabular}{l | cc }
%		\toprule
%		Data &
%		\multicolumn{2}{c}{server room} \\
%	    \midrule
%		\diagbox[height=2em]{Method}{Metric}
%		& RMSE & MAE
%		\\ \midrule
%		\cpals~\cite{harshman1970foundations}
%		& 0.625 & 0.409 \\ [0.3em]
%		CoSTCo~\cite{liu2019costco}
%		& 1.534 & 1.041 \\ [0.3em]
%		TRMF~\cite{yu2016temporal}
%		& 4.249 & 2.917 \\ [0.3em]
%		NTF~\cite{wu2019neural}
%		& 4.541 & 3.490 \\ [0.3em]
%		\midrule
%		\methodz
%		& \underline{0.401} & \underline{0.266} \\ [0.3em]
%		\bf{\method}
%		&  \bf{0.347} & \bf{0.233}
%		\\
%	\bottomrule
%	\end{tabular}
%	\label{tab:appendix_exp}
%\end{table}

\begin{figure*}
	\addvspace{6mm}
	\centering
    \includegraphics[width=0.25\linewidth]{./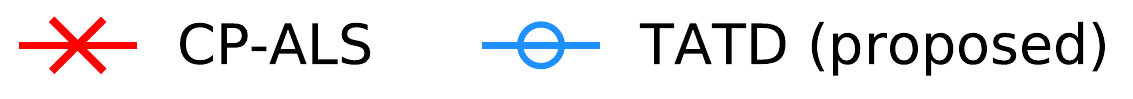}\vspace{1mm}\\
    \subfigure[Sparsity]{
        \includegraphics[width=0.3\linewidth]{./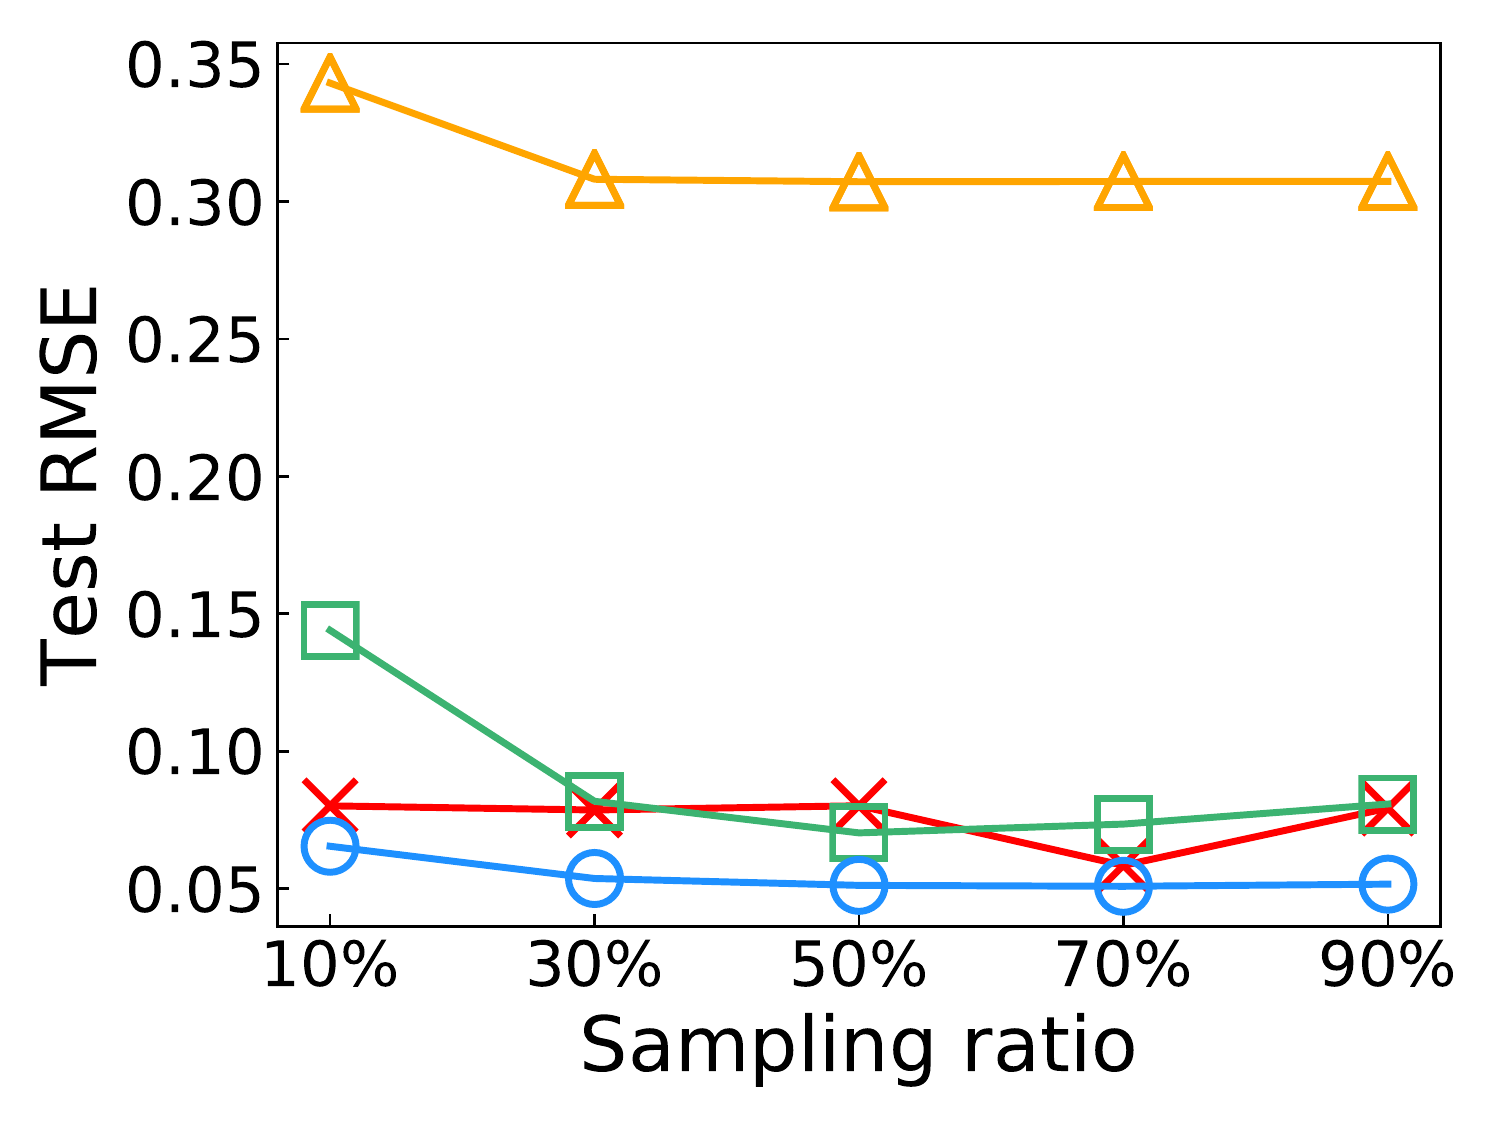}
    }
    \subfigure[Penalty]{
        \includegraphics[width=0.3\linewidth]{./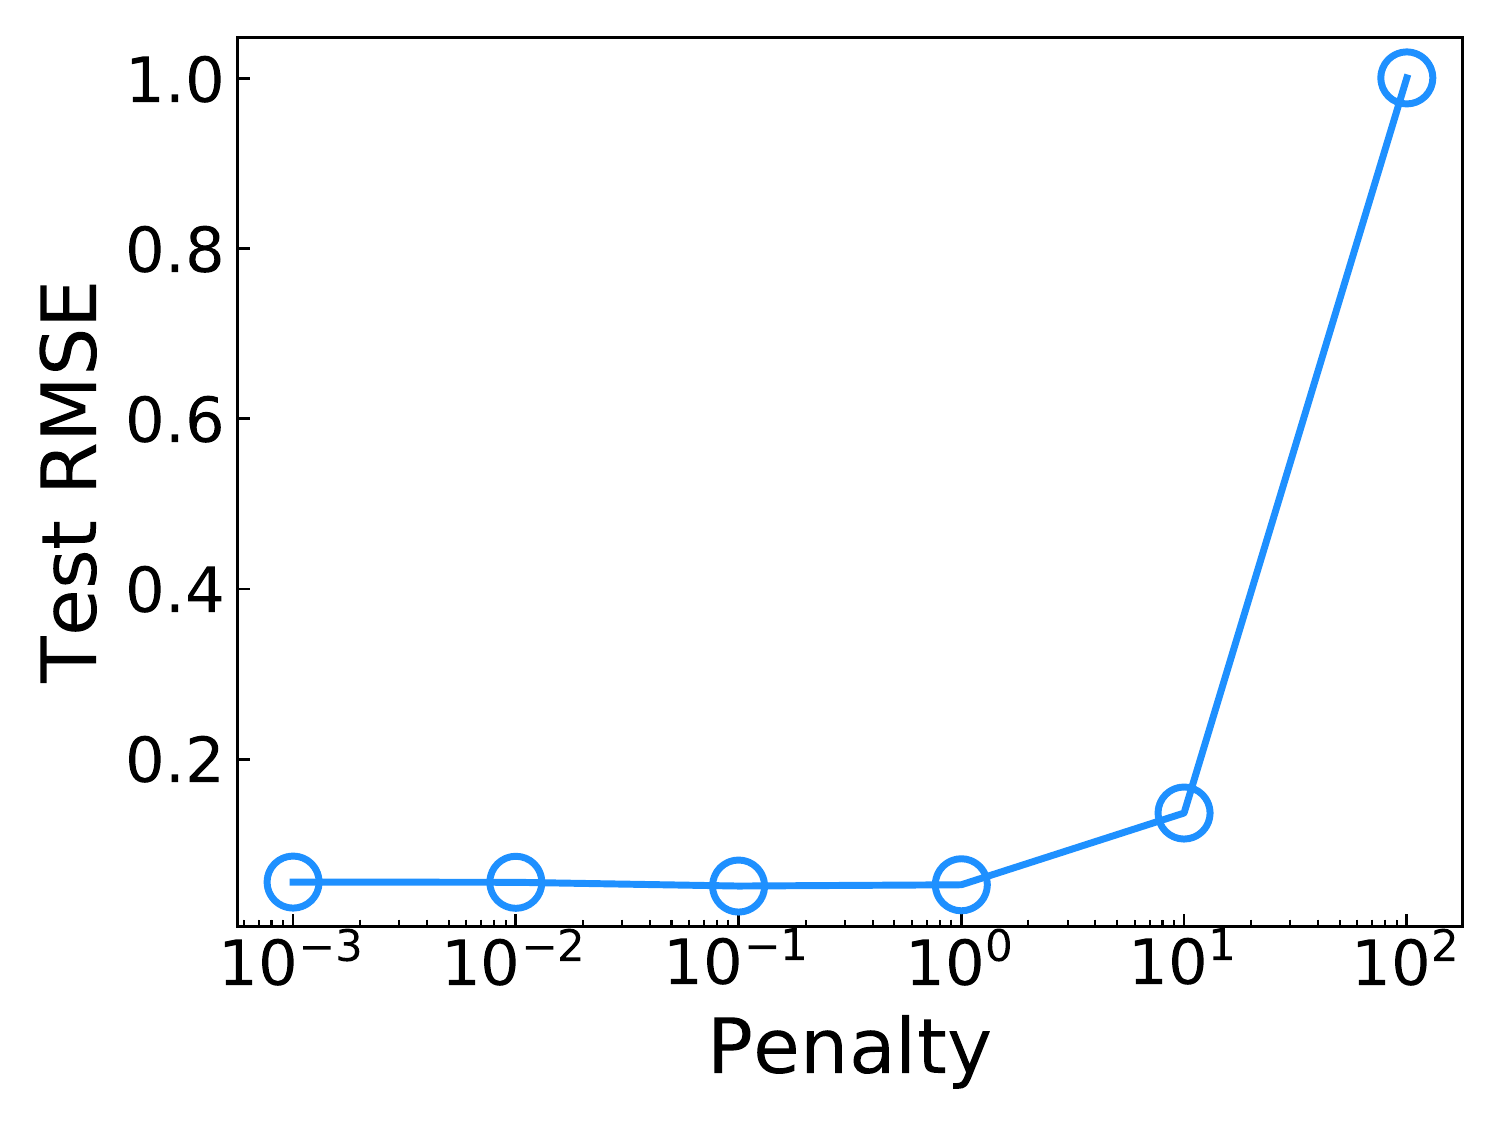}
    }
    \subfigure[Rank]{
        \includegraphics[width=0.3\linewidth]{./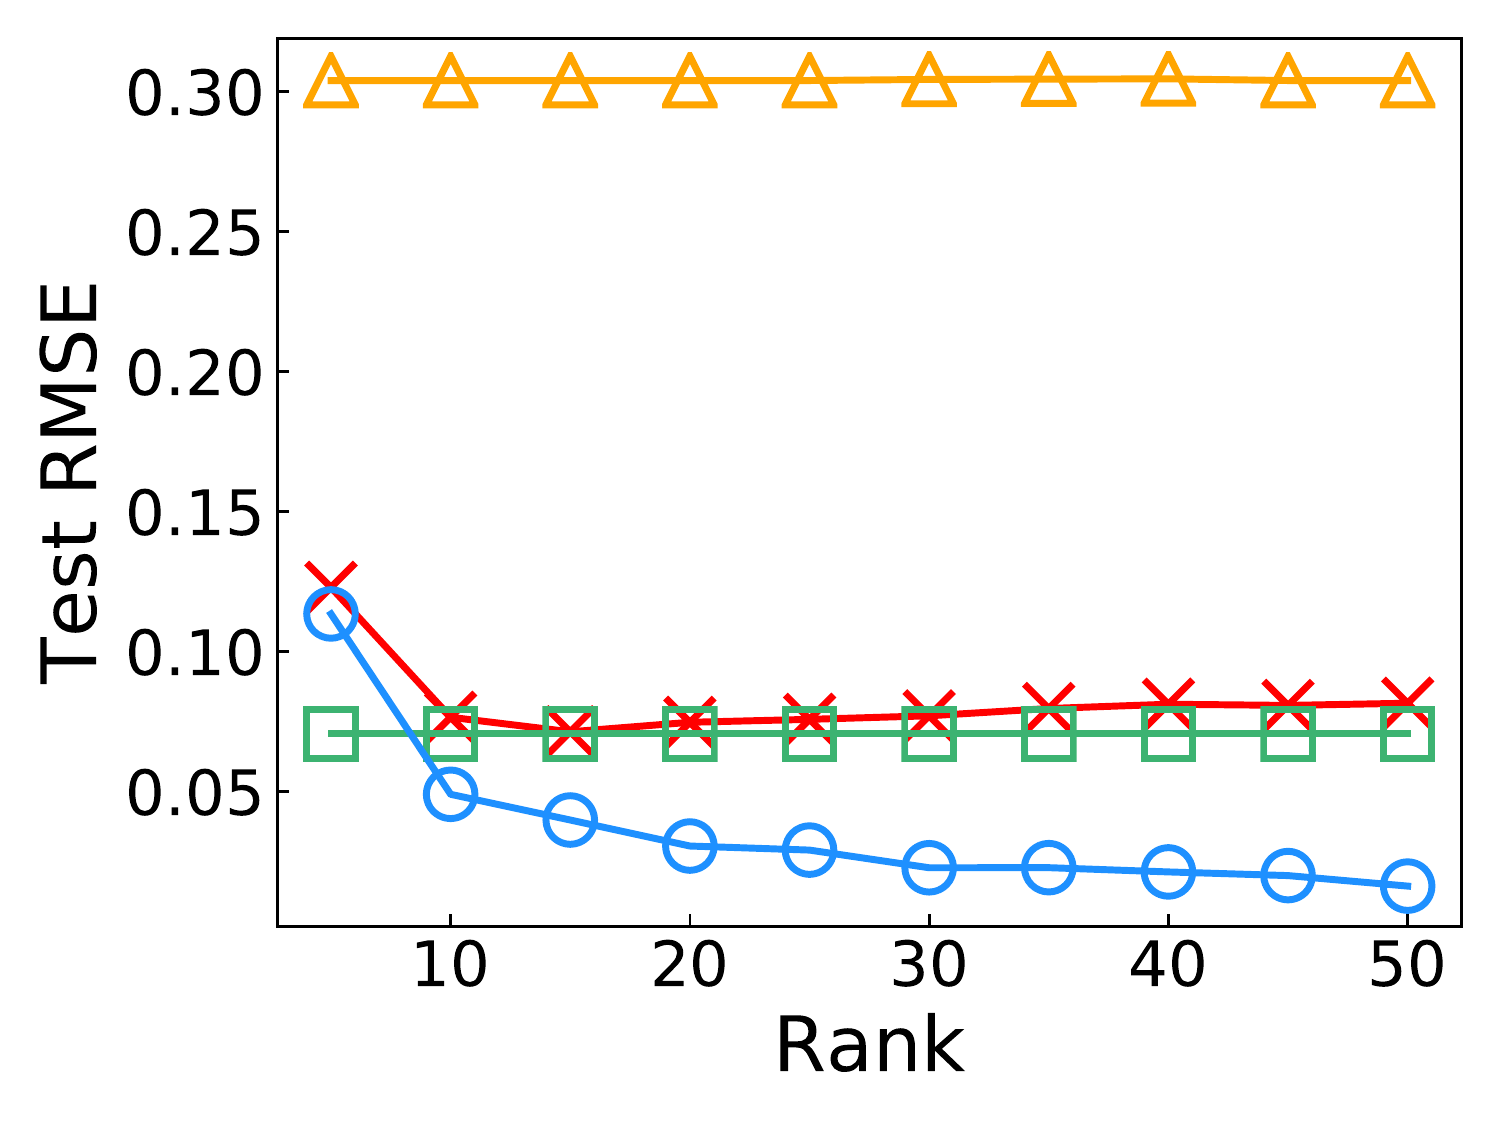}
    }
    \caption{\label{fig:sparsity_ratio_1}
    Test RMSE of \method and the best competitor CP-ALS for three experiments:
    (a) sampling ratio, (b) penalty, and (c) rank.
    }
\end{figure*}
